# Supplementary material for: Fragmentation and optimal liquidity supply on decentralized exchanges
Source: arXiv:2307.13772 source file (2024-05-21)
Supplement: Supplementary file 2 [file proof_rebalance_old.tex]

\noindent\textbf{\large Lemma \ref{lem:sort}}
\begin{proof}
Suppose that $\LP$s with $q_i\leq\qmg$ post liquidity on the low-fee pool and all $\LP$s with $q_i>\qmg$ choose the high-fee pool. For an $\LP$ with endowment $\tilde{q}<\qmg$, submitting liquidity to pool $L$ yields a lower expected revenue since
\begin{equation*}
    \pi_L-\pi_H=\frac{1}{d_H d_L}\left[\left(d_H \ell - d_L h\right) \tilde{q} - \Gamma \left(d_H-d_L\right)\right] < 0.
\end{equation*}
The result follows. \end{proof}

\bigskip
\noindent \textbf{\large Proposition \ref{prop:equilibria}}
\begin{proof}
We rewrite equation \eqref{eq:pi_diff} as
\begin{align}\label{eq:pi_diff_v2}
    \pi_\ell-\pi_h    &=\frac{1}{\lambda d_h d_\ell}\left[q_i\left(h \times \left(\frac{\qmg}{Q}\right)^{\frac{\lambda}{\theta}\frac{Q}{Q-1}} -\left(h-l\right)\right) -\Gamma \left(\frac{\qmg}{Q}\right)^{\frac{\lambda}{\theta}\frac{Q}{Q-1}} \right]. 
\end{align}

If the coefficient of $q_i$ in \eqref{eq:pi_diff_v2} is negative, that is $h \times \left(\frac{\qmg}{Q}\right)^{\frac{\lambda}{\theta}\frac{Q}{Q-1}} -\left(h-l\right)\leq 0$, then $\pi_\ell-\pi_h<0$ and all $\LP$s optimally choose to post liquidity on pool $H$. A necessary condition for a fragmented equilibrium is therefore that
\begin{equation}\label{eq:denominator}
   f_1\left(\qmg\right) \coloneqq h \times \left(\frac{\qmg}{Q}\right)^{\frac{\lambda}{\theta}\frac{Q}{Q-1}} -\left(h-\ell\right)>0
\end{equation}
The function $f_1\left(\qmg\right)$ increases in $\qmg$, and therefore it has at most one root $q_r$ in $\left[1,Q\right]$. Since $f_1\left(Q\right)=\ell>0$, it follows that $q_r\in\left[1,Q\right)$ if and only if
\begin{equation}
    f_1\left(1\right)<0 \Rightarrow \frac{h-l}{h} Q^{\frac{\lambda}{\theta}\frac{Q}{Q-1}} > 1
\end{equation}

Second, in any fragmented market equilibrium, the marginal $\LP$ is indifferent between providing liquidity on the $L$ or $H$ pool. Equivalently, the marginal trader solves $\pi_\ell-\pi_h=0$, which from equation \eqref{eq:mg_eq} translates to a solution of
\begin{equation}\label{eq:reactfunct_proof}
    f_2\left(\qmg\right) \coloneqq \Gamma \frac{\qmg^{\frac{\lambda}{\theta}\frac{Q}{Q-1}} \times Q^{-\frac{\lambda}{\theta}\frac{Q}{Q-1}}}{h\left[\qmg^{\frac{\lambda}{\theta}\frac{Q}{Q-1}} \times Q^{-\frac{\lambda}{\theta}\frac{Q}{Q-1}}\right]-\left(h-\ell\right)} - \qmg =0.
\end{equation}
We show that  $f_2\left(\cdot\right)$ monotonically decreases in $\qmg$ since
\begin{equation}\label{eq:mon_f2}
    \frac{\partial f_2\left(\qmg\right)}{\partial \qmg}=-\Gamma\frac{\lambda  (h-l) Q^{\frac{\lambda  Q}{\theta  (Q-1)}+1} \qmg^{\frac{\lambda  Q}{\theta  (Q-1)}-1}}{\theta  (Q-1) \left((l-h) Q^{\frac{\lambda  Q}{\theta  (Q-1)}}+h \qmg^{\frac{\lambda  Q}{\theta  (Q-1)}}\right)^2}-1<0,
\end{equation}
and therefore it has at most one root. That is, if a fragmented market equilibrium exists, then it is unique.

To complete the proof, we consider two cases. First, let $\frac{h-l}{h} Q^{\frac{\lambda}{\theta}\frac{Q}{Q-1}} > 1$ such that $q_r>1$. For a belief $\qmg<q_r<Q$, liquidity providers optimally choose pool $H$ -- which is equivalent to having an outcome in which the marginal trader is $\qmg=Q$. Therefore, there is no fulfilled expectation equilibrium on $\left[1,q_r\right]$ in which beliefs match outcomes. From the intermediate value theorem and monotonicity of $f_2\left(\qmg\right)$, there is exactly one root of $f_2\left(\qmg\right)$ on $\left(q_r,Q\right]$ since 
\begin{equation}
    \underbrace{\frac{\Gamma}{\ell} - Q}_{<0} = f_2\left(Q\right)  < f_2\left(\qmg\right) < \lim_{\qmg \downarrow q_r} f_2\left(\qmg\right) = \infty.
\end{equation}
Therefore, for $\frac{h-l}{h} Q^{\frac{\lambda}{\theta}\frac{Q}{Q-1}} > 1$ there is one unique equilibrium with fragmented markets.

Second, consider the case where $\frac{h-l}{h} Q^{\frac{\lambda}{\theta}\frac{Q}{Q-1}} \leq 1$ such that $q_r<1$. In this case the reaction function $f_2\left(\qmg\right)$ is decreasing and has no discontinuities. If $\frac{\Gamma}{h}>1$ such that the marginal $\LP$ earns zero expected profit, it follows from the intermediate value theorem and monotonicity of $f_2$ that there is a unique fragmented equilibrium since $f_2\left(\frac{\Gamma}{h}\right)>0$ and $f_2\left(Q\right)<0$. 

Otherwise -- if $\frac{\Gamma}{h}<1$ -- a necessary and sufficient condition for a unique interior root is that $f_2\left(1\right)>0$ or, equivalently, that
\begin{equation}\label{eq:cond_frag}
    \frac{\Gamma}{h}>1-\frac{h-l}{h} Q^{\frac{\lambda}{\theta}\frac{Q}{Q-1}}.
\end{equation}
If \eqref{eq:cond_frag} does not hold, then $f_2\left(1\right)<0$ which, from monotonicity, implies that $f_2\left(\qmg\right)<0$ for all $\qmg\in\left[1,Q\right]$. In this case, the unique equilibrium is that all liquidity providers deposit their endowments on pool $L$. \end{proof}

\noindent \textbf{\large Corollary \ref{cor:comp_stat}}
\begin{proof}
From the implicit function theorem, 
\begin{equation}
    \frac{\partial \qmg^\star}{\partial x}=-\left(\frac{\partial f_2}{\partial x}\right)^{-1} \frac{\partial f_2}{\partial \qmg}.
\end{equation}
Since from equation \eqref{eq:mon_f2} $f_2\left(\cdot\right)$ decreases in $\qmg$, it follows that the sign of $\frac{\partial \qmg^\star}{\partial x}$ is the same as the sign of $\frac{\partial f_2}{\partial x}$, which significantly simplifies the task.

First, we note that
\begin{equation}
    \frac{\partial f_2}{\partial \Gamma}=\frac{\qmg^{\frac{\lambda}{\theta}\frac{Q}{Q-1}} \times Q^{-\frac{\lambda}{\theta}\frac{Q}{Q-1}}}{h\left[\qmg^{\frac{\lambda}{\theta}\frac{Q}{Q-1}} \times Q^{-\frac{\lambda}{\theta}\frac{Q}{Q-1}}\right]-\left(h-\ell\right)}>0,
\end{equation}
and therefore $\qmg^\star$ increases in $\Gamma$. Second,
\begin{align}
    \frac{\partial f_2}{\partial \lambda}=\frac{\Gamma  (h-l) Q^{\frac{\lambda  Q}{\theta  (Q-1)}+1} (\log (Q)-\log (\qmg)) \qmg^{\frac{\lambda  Q}{\theta  (Q-1)}}}{\theta  (Q-1) \left((l-h) Q^{\frac{\lambda  Q}{\theta  (Q-1)}}+h \qmg^{\frac{\lambda  Q}{\theta  (Q-1)}}\right)^2}>0,
\end{align}
since $\qmg<Q$. Therefore, $\qmg^\star$ increases in $\lambda$. Third,
\begin{equation}
    \frac{\partial f_2}{\partial \theta}=-\frac{\Gamma  \lambda  (h-l) Q^{\frac{\lambda  Q}{\theta  (Q-1)}+1} (\log (Q)-\log (\qmg)) \qmg^{\frac{\lambda  Q}{\theta  (Q-1)}}}{(Q-1) \left(\theta  (h-l) Q^{\frac{\lambda  Q}{\theta  (Q-1)}}-h \theta  \qmg^{\frac{\lambda  Q}{\theta  (Q-1)}}\right)^2}<0,
\end{equation}
which implies that $\qmg^\star$ decreases in $\theta$. Fourth,
\begin{equation}
    \frac{\partial f_2}{\partial Q}=\frac{\Gamma  \lambda  (h-l) Q^{\frac{\lambda  Q}{\theta -\theta  Q}} (Q-\log (Q)+\log (\qmg)-1) \qmg^{\frac{\lambda  Q}{\theta -\theta  Q}}}{\theta  (Q-1)^2 \left((l-h) \qmg^{\frac{\lambda  Q}{\theta -\theta  Q}}+h Q^{\frac{\lambda  Q}{\theta -\theta  Q}}\right)^2}>0,
\end{equation}
since $Q-\log (Q)+\log (\qmg)-1>Q-\log(Q)-1>0$, where the latter inequality stems from $Q>1$. Therefore, $\qmg^\star$ increases in $Q$.

Finally, we compute partial derivatives with respect to pool fees $h$ and $l$. That is
\begin{align}
    \frac{\partial f_2}{\partial h}=\frac{\Gamma  Q^{-\frac{\lambda  Q}{(Q-1)\theta}} \left(\qmg^{-\frac{\lambda  Q}{(Q-1)\theta}}-Q^{-\frac{\lambda  Q}{(Q-1)\theta}}\right)}{\left((l-h) \qmg^{\frac{\lambda  Q}{\theta -\theta  Q}}+h Q^{\frac{\lambda  Q}{\theta -\theta  Q}}\right)^2}>0
\end{align}
since $\qmg<Q$ and $\frac{\lambda  Q}{(Q-1)\theta}>0$; further,
\begin{align}
    \frac{\partial f_2}{\partial l}=-\frac{\Gamma  Q^{\frac{\lambda  Q}{\theta -\theta  Q}} \text{qm}^{\frac{\lambda  Q}{\theta  (Q-1)}}}{\left(h \left(Q^{\frac{\lambda  Q}{\theta -\theta  Q}} \text{qm}^{\frac{\lambda  Q}{\theta  (Q-1)}}-1\right)+l\right)^2}<0.
\end{align}

\end{proof}

\noindent \textbf{\large Corollary \ref{cor:comp_stat_ms}}
\begin{proof}
The comparative statics with respect to $\lambda$, $\theta$, and $\ell$ follow immediately from Corollary \ref{cor:comp_stat} and the fact that $w_L$ decreases in $\qmg$.

If $\frac{\Gamma}{h}>1$ such that $\underline{q}=\frac{\Gamma}{h}$, then the partial derivative of $w_L$ with respect to $h$ is
\begin{equation}
    \frac{\partial w_L}{\partial h}=-\frac{\left(\log Q - \log \qmg\right) \qmg + h \left(\log \qmg-\log \frac{\Gamma}{h}\right)\frac{\partial \qmg}{\partial h}}{h\left(\log Q - \log \qmg\right)^2\qmg},
\end{equation}
which is positive since from Corollary \ref{cor:comp_stat} we have that $\frac{\partial \qmg}{\partial h}>0$.
Otherwise, if  $\frac{\Gamma}{h}>1$ such that $\underline{q}=1$, then
\begin{equation}
    \frac{\partial w_L}{\partial h}=-\frac{\partial \qmg}{\partial h} \frac{1}{\log Q \qmg}<0.
\end{equation}

The partial derivative of $w_L$ with respect to $Q$ is
\begin{equation}
    \frac{\partial w_L}{\partial h}=-\frac{\left(\log \qmg - \log \underline{q}\right) \qmg - Q \left(\log Q - \log \underline{q}\right)\frac{\partial \qmg}{\partial Q}}{Q\left(\log Q - \log \underline{q}\right)^2 \qmg},
\end{equation}


\end{proof}
