# Supplementary material for: Fragmentation and optimal liquidity supply on decentralized exchanges
Source: arXiv:2307.13772 source file (2024-05-21)
Supplement: Supplementary file 3 [file todo.tex]

\section{To do list}

\begin{itemize}
    \item Conjecture: there is no single-fee liquidity pool that achieves higher LP participation and lower transaction costs for liquidity traders. To prove?
    \item Corollary: a menu of fees improves market quality by encouraging LP participation. The correct counter-factual is not to compare high-fee pool LPs to low-fee pool LPs but low-endowment LPs in a world with fragmentation (where they can supply liquidity and earn positive returns) with a world without fragmentation where they are shut out of the market.
    \item Address the issue of adverse selection. 
        \begin{enumerate}
            \item Alternative channel: a higher gas fee discourages arbitrageurs, who first forego arbitrage opportunities on high-fee pools. Therefore, a higher gas fee is disproportionately better for high-fee LPs, which maps to our migration result too.
            \item Occam's Razor: We do not need to have adverse selection to generate our result, so what does it add?
            \item We already control for volatility. Control for impermanent loss? Control for interaction between gas price and impermanent loss? 
        \end{enumerate}
\end{itemize}

\subsection{Theory}

\begin{enumerate}
    \item Let $\Theta>\frac{Q}{Q-1}\log Q$ denote the trade size for the large LT, and let $g$ denote the gains from trade.
    \item For a sequence of $N$ pools indexed by $k$, let $f_k$ be the liquidity fee on pool $k$ and $\mathcal{L}_k$ the equilibrium liquidity on pool $k$.
    \item Define the \textbf{implementation shortfall} as follows:
    \begin{equation}
        \text{IS}=\underbrace{\sum_k f_k \mathcal{L}_k}_\text{trading cost} + \underbrace{g \left(\theta - \sum_k \mathcal{L}_k\right)}_\text{unrealized gains}
    \end{equation}
\end{enumerate}
